# Supplementary material for: CodeCloak: A Method for Evaluating and Mitigating Code Leakage by LLM Code Assistants
Source: arXiv:2404.09066 source file (2024-10-29)
Supplement: Supplementary file 1 [file appendix.tex]

\onecolumn
\section{\label{sec:eval}GitHub Dataset}
In Table~\ref{tab:GitHub_Repositories} we list the repositories used in our experiments (we randomly selected 20 repositories with the condition of 3-4 files in each repository). 

\begin{table*}[htbp]
\centering
\caption{GitHub repositories used in our experiments}
\label{tab:GitHub_Repositories}
\scalebox{0.7}{
\begin{tabular}{cl}
\toprule
\# & Github File Path  \\ 
\midrule
1 & \url{https://github.com/DannyPol/flatcam/blob/master/Bookmark.py} \\
  & \url{https://github.com/DannyPol/flatcam/blob/master/FlatCAM.py} \\
  & \url{https://github.com/DannyPol/flatcam/blob/master/Utils/remove_bad_profiles_from_pictures.py} \\
  & \url{https://github.com/DannyPol/flatcam/blob/master/Utils/vispy_example.py} \\
\addlinespace
2 & \url{https://github.com/neal-hub/nvda-test/blob/master/appveyor/mozillaSyms.py} \\
  & \url{https://github.com/neal-hub/nvda-test/blob/master/devDocs/conf.py} \\
  & \url{https://github.com/neal-hub/nvda-test/blob/master/extras/controllerClient/x86/example_python.py} \\
  & \url{https://github.com/neal-hub/nvda-test/blob/master/keyCommandsDoc.py} \\
\addlinespace
3 & \url{https://github.com/vkumarma/Complete-Interpreter/blob/main/evaluator.py} \\
  & \url{https://github.com/vkumarma/Complete-Interpreter/blob/main/main.py} \\
  & \url{https://github.com/vkumarma/Complete-Interpreter/blob/main/parser.py} \\
\addlinespace
4 & \url{https://github.com/leelige/mindspore/blob/master/official/audio/melgan/ascend310_infer/preprocess.py} \\
  & \url{https://github.com/leelige/mindspore/blob/master/official/audio/melgan/eval.py} \\
  & \url{https://github.com/leelige/mindspore/blob/master/official/audio/melgan/export.py} \\
  & \url{https://github.com/leelige/mindspore/blob/master/official/audio/melgan/src/dataset.py} \\
\addlinespace
5 & \url{https://github.com/jmerizia/parallel-pytorch/blob/main/examples/train_minGPT.py} \\
  & \url{https://github.com/jmerizia/parallel-pytorch/blob/main/parallel_pytorch/data.py} \\
  & \url{https://github.com/jmerizia/parallel-pytorch/blob/main/parallel_pytorch/layers.py} \\
\addlinespace
6 & \url{https://github.com/gzpyy/qlib/blob/main/docs/conf.py} \\
  & \url{https://github.com/gzpyy/qlib/blob/main/examples/benchmarks/LightGBM/features_resample_N.py} \\
  & \url{https://github.com/gzpyy/qlib/blob/main/examples/benchmarks/LightGBM/features_sample.py} \\
  & \url{https://github.com/gzpyy/qlib/blob/main/examples/benchmarks/LightGBM/multi_freq_handler.py} \\
\addlinespace
7 & \url{https://github.com/pennfranc/hypnettorch/blob/master/docs/source/conf.py} \\
  & \url{https://github.com/pennfranc/hypnettorch/blob/master/hypnettorch/data/__init__.py} \\
  & \url{https://github.com/pennfranc/hypnettorch/blob/master/hypnettorch/data/celeba_data.py} \\
\addlinespace
8 & \url{https://github.com/hwaipy/InteractionFreeNode/blob/master/appllication/Scripts/PackageAndPublish.py} \\
  & \url{https://github.com/hwaipy/InteractionFreeNode/blob/master/appllication/Scripts/Uploader.py} \\
  & \url{https://github.com/hwaipy/InteractionFreeNode/blob/master/runtime/python/Lib/__future__.py} \\
\addlinespace
9 & \url{https://github.com/mgelbart/ray/blob/master/.buildkite/copy_files.py} \\
  & \url{https://github.com/mgelbart/ray/blob/master/ci/build/build-docker-images.py} \\
  & \url{https://github.com/mgelbart/ray/blob/master/ci/build/build-multinode-image.py} \\
  & \url{https://github.com/mgelbart/ray/blob/master/ci/build/get_build_info.py} \\
\addlinespace
10 & \url{https://github.com/sowmyav27/rancher/blob/release/v2.7/tests/integration/setup.py} \\
   & \url{https://github.com/sowmyav27/rancher/blob/release/v2.7/tests/integration/suite/alert_common.py} \\
   & \url{https://github.com/sowmyav27/rancher/blob/release/v2.7/tests/integration/suite/cluster_common.py} \\
\addlinespace
11 & \url{https://github.com/BearerPipelineTest/synapse-1/blob/develop/.ci/scripts/calculate_jobs.py} \\
   & \url{https://github.com/BearerPipelineTest/synapse-1/blob/develop/.ci/scripts/postgres_exec.py} \\
   & \url{https://github.com/BearerPipelineTest/synapse-1/blob/develop/contrib/cmdclient/console.py} \\
   & \url{https://github.com/BearerPipelineTest/synapse-1/blob/develop/contrib/cmdclient/http.py} \\
\addlinespace
12 & \url{https://github.com/ebezzam/PolyatomicFW_SPL/blob/main/example.py} \\
   & \url{https://github.com/ebezzam/PolyatomicFW_SPL/blob/main/frank_wolfe.py} \\
   & \url{https://github.com/ebezzam/PolyatomicFW_SPL/blob/main/plot_comparison_cs.py} \\
   & \url{https://github.com/ebezzam/PolyatomicFW_SPL/blob/main/plot_saved_results.py} \\
\addlinespace
13 & \url{https://github.com/MelisaDev/melisa/blob/master/docs/source/conf.py} \\
   & \url{https://github.com/MelisaDev/melisa/blob/master/docs/source/extensions/attributable.py} \\
   & \url{https://github.com/MelisaDev/melisa/blob/master/melisa/__init__.py} \\
   & \url{https://github.com/MelisaDev/melisa/blob/master/melisa/cache.py} \\
\addlinespace
14 & \url{https://github.com/corey-sobel/qcore/blob/master/qcore/__init__.py} \\
   & \url{https://github.com/corey-sobel/qcore/blob/master/qcore/asserts.py} \\
   & \url{https://github.com/corey-sobel/qcore/blob/master/qcore/caching.py} \\
   & \url{https://github.com/corey-sobel/qcore/blob/master/qcore/debug.py} \\
\addlinespace
15 & \url{https://github.com/los-verdes/lv-event-pagenerator/blob/main/events_page/apis/__init__.py} \\
   & \url{https://github.com/los-verdes/lv-event-pagenerator/blob/main/events_page/apis/calendar.py} \\
   & \url{https://github.com/los-verdes/lv-event-pagenerator/blob/main/events_page/apis/constants.py} \\
   & \url{https://github.com/los-verdes/lv-event-pagenerator/blob/main/events_page/apis/drive.py} \\
\addlinespace
16 & \url{https://github.com/isabella232/pynacl/blob/main/docs/conf.py} \\
   & \url{https://github.com/isabella232/pynacl/blob/main/docs/vectors/python/argondriver.py} \\
   & \url{https://github.com/isabella232/pynacl/blob/main/release.py} \\
   & \url{https://github.com/isabella232/pynacl/blob/main/setup.py} \\
\addlinespace
17 & \url{https://github.com/VITA-Group/Peek-a-Boo/blob/main/bop.py} \\
   & \url{https://github.com/VITA-Group/Peek-a-Boo/blob/main/generator.py} \\
   & \url{https://github.com/VITA-Group/Peek-a-Boo/blob/main/logger.py} \\
   & \url{https://github.com/VITA-Group/Peek-a-Boo/blob/main/main_cifar.py} \\
\addlinespace
18 & \url{https://github.com/29riyasaxena/MDF/blob/main/docs/generate.py} \\
   & \url{https://github.com/29riyasaxena/MDF/blob/main/docs/sphinx/source/conf.py} \\
   & \url{https://github.com/29riyasaxena/MDF/blob/main/examples/ACT-R/addition.py} \\
   & \url{https://github.com/29riyasaxena/MDF/blob/main/examples/ACT-R/count.py} \\
\addlinespace
19 & \url{https://github.com/artigianitecnologici/marrtino_apps/blob/master/actions/actionproxy.py} \\
   & \url{https://github.com/artigianitecnologici/marrtino_apps/blob/master/actions/conditionproxy.py} \\
   & \url{https://github.com/artigianitecnologici/marrtino_apps/blob/master/actions/frontobstacle_conditionproxy.py} \\
   & \url{https://github.com/artigianitecnologici/marrtino_apps/blob/master/actions/movebase_actionproxy.py} \\
\addlinespace
20 & \url{https://github.com/TolyaTalamanov/open_model_zoo/blob/master/ci/check-basics.py} \\
   & \url{https://github.com/TolyaTalamanov/open_model_zoo/blob/master/ci/check-documentation.py} \\
   & \url{https://github.com/TolyaTalamanov/open_model_zoo/blob/master/ci/check-release-readiness.py} \\
   & \url{https://github.com/TolyaTalamanov/open_model_zoo/blob/master/ci/documentation_updater/documentation_updater.py} \\
\bottomrule
\end{tabular}}
\end{table*}

\clearpage

\section{\label{sec:examples}Prompts Examples}

%EDEN - ADD HERE SHORT DESCRIPTION OF THE FILE
In the \texttt{Reconstruction\_model\_input-output\_example.pdf} file provided in the supplementary material, we present an example of the input and the output of the Reconstruction model. 
The code segments provided in this file was extracted from the prompts of \texttt{addition.py} file are after data preparation phase. 
These segments are arranged according to their original sequence. 
At the end of the file, we present the reconstructed code by  of the \texttt{addition.py} file (using ChatGPT4). 
In this case, the Reconstruction model was able to reconstruct the whole code correctly, demonstrating a scenario of 100\% code leakage. 

\section{\label{sec:examples}Examples of Prompts and Code Suggestions}

In the \texttt{CodeCloak\_prompt\_manipulations\_and\_responses\_examples.pdf} file provided in the supplementary material, we present a list of examples featuring original prompts, suggestions, and the manipulated prompts and suggestions following application of our \MethodName DRL agent. 
The code assistant utilized for generating the suggestions is StarCoder.

%\clearpage
\section{\label{sec:heatmap}CodeCloak Action Distribution Heatmap}
The heat map in Figure~\ref{fig:heatmap} presents the distribution of different manipulations/actions ($x$-axis) chosen by \MethodName across various time steps (y-axis) during the evaluation process. 
Note that the heatmap refers to sequences of manipulations of variable length.

\begin{figure}[h]
    \centering
\includegraphics[width=0.8\linewidth]{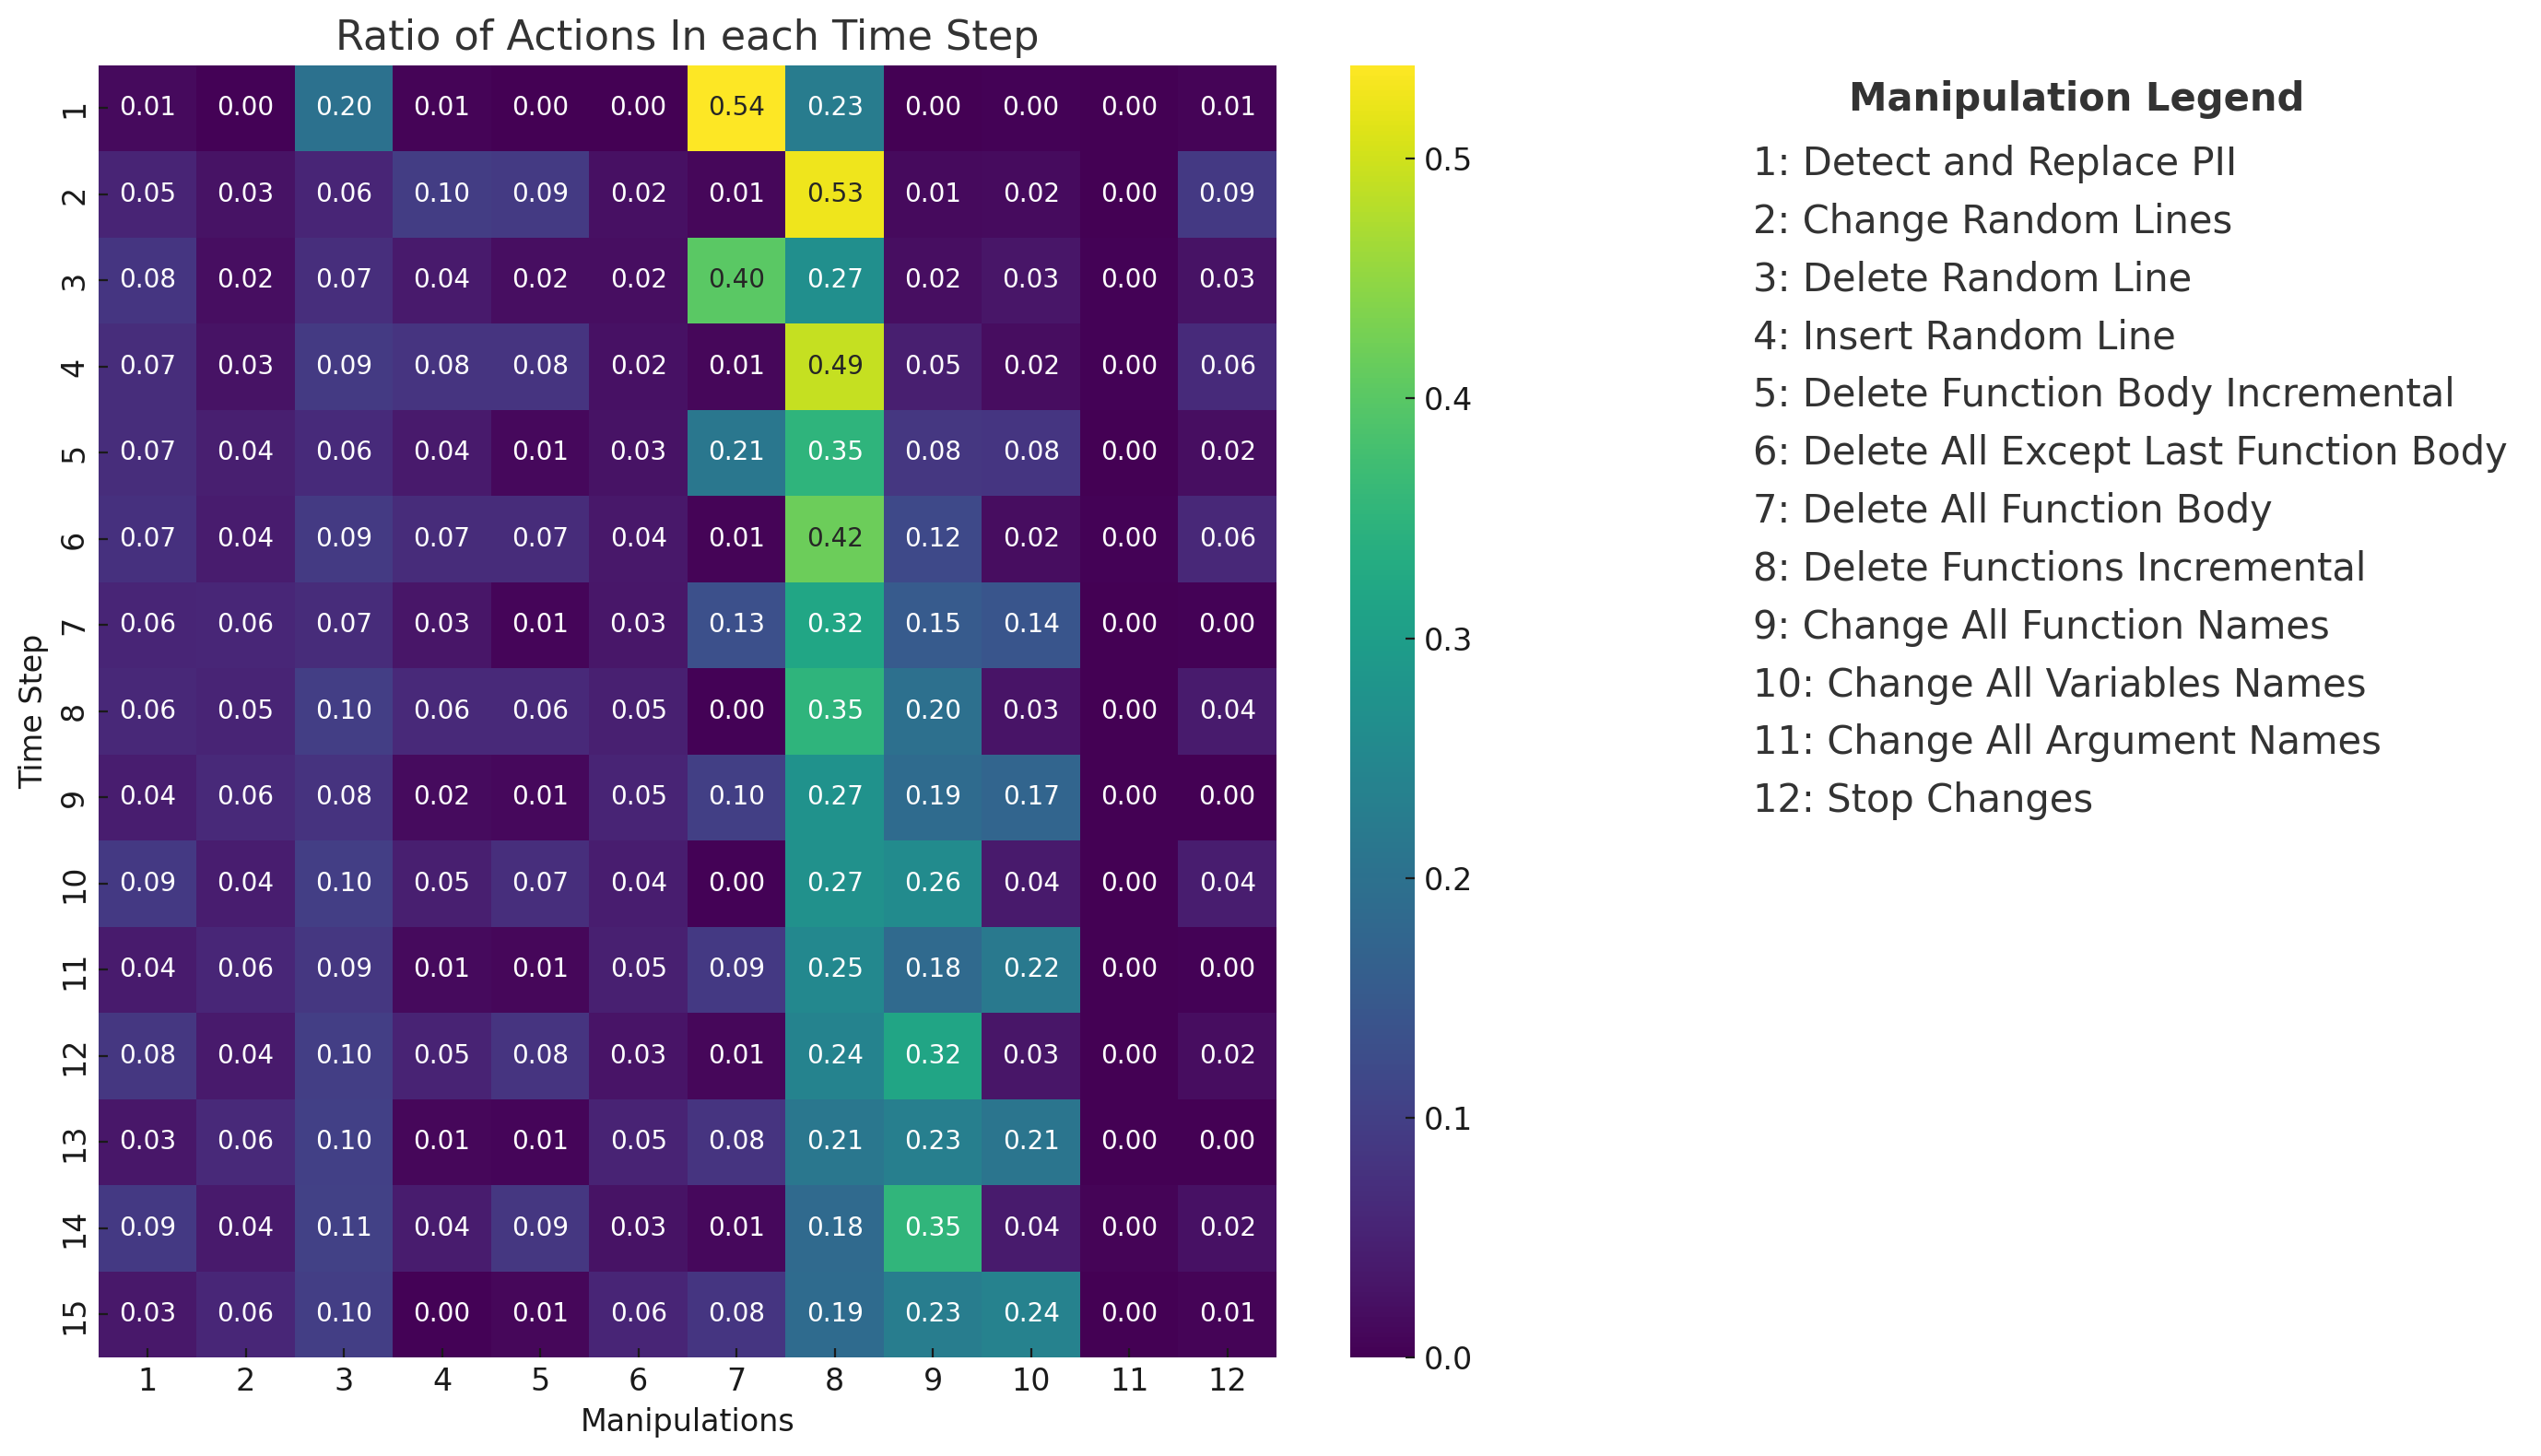}
    %\vspace{-0.3cm}
    \caption{CodeCloak Action Distribution Heatmap.}
    \label{fig:heatmap}
\end{figure}

\newpage
\section{\label{sec:hyper_parameters}HyperParmameters for training CodeCloak}
The table below provides the training details for \MethodName. 
In addition, We also adopt parallel environment in our training process (eight environments). 
We have noticed that large size of parallel environments helped for our training process. 

\begin{table}[h]
\centering
\begin{tabular}{l|l}
\hline
\textbf{Hyperparameter} & \textbf{Value} \\ \hline
Learning Rate & 0.00025 \\
Time Limit (per episode) & 15 \\
Gamma (Discount Factor) & 0.99 \\
GAE Lambda & 0.95 \\
N Steps & 128 \\
Batch Size & 64 \\
Clip Range & 0.2 \\
Entropy Coefficient & 0.01 \\
Policy Net Arch & \begin{tabular}[c]{@{}l@{}}Policy Network: [256, 256, 256, 128],\\ Value Network: [256, 256, 256, 128]\end{tabular} \\ \hline
\end{tabular}
\caption{Hyperparameters and Policy Configuration for Training CodeCloak}
\label{tab:hyperparameters_policy}
\end{table}

\section{\label{sec:Heatmap}Examples of Prompts and Code Suggestions}
